# Supplementary material for: Learning physics-informed simulation models for soft robotic manipulation: A case study with dielectric elastomer actuators
Source: arXiv:2202.12977 source file (2022-07-16)
Supplement: Supplementary file 1 [file Appendix_2.tex]

%%%%%%%%%%%%%%%%%%%%%%%%%%%%%%%%%%%%%%%%%%%%%%%%%%%%%%%%%%%%%%%%%%%%%%%%%%%%%%%%
%%%%%%%%%%%%%%%%%%%%%%%%%%%%%%%%%%%%%%%%%%%%%%%%%%%%%%%%%%%%%%%%%%%%%%%%%%%%%%%%
\section{Dielectric Elastomers Actuator}
\label{sec:DEA}
%%%%%%%%%%%%%%%%%%%%%%%%%%%%%%%%%%%%%%%%%%%%%%%%%%%%%%%%%%%%%%%%%%%%%%%%%%%%%%%%
%%%%%%%%%%%%%%%%%%%%%%%%%%%%%%%%%%%%%%%%%%%%%%%%%%%%%%%%%%%%%%%%%%%%%%%%%%%%%%%%

Dielectric Elastomers Actuators (DEA) are deformable actuators used in soft robotic manipulation. Dielectric elastomers (DE) are a type of electroactive polymers that produce mechanical strain under the influence of electric voltage, and thus a dielectric elastomer membrane expands its area when a voltage is applied across its thickness~\cite{Pelrine_2000_DE}. Such ability to convert electrical energy to mechanical energy makes them ideal for developing actuators for soft robots~\cite{Youn_2020_review,Ron_2002_muscleacutators}. 

A typical DEA consists of polymer film that is coated with compliant electrodes on both sides. Multiple layers of active and inactive DE membranes can be stacked to design unimorph or bimorph DEA.~\fref{fig:DEADiagrams}a) shows unimorph DEA, with one active and one constraining layer. The active layer expands under externally applied voltage causing the bending motion.

%%%%%%%%%%%%%%%%%%%%%%%%%%%%%%%%%%%%%%%%%%%%%%%%%%%%%%%%%%%%%%%%%%%%%%%%%%%%%%%%
\paragraph{DE material}
\label{sec:DEMaterialdef}
%%%%%%%%%%%%%%%%%%%%%%%%%%%%%%%%%%%%%%%%%%%%%%%%%%%%%%%%%%%%%%%%%%%%%%%%%%%%%%%%
A DE material exhibits the effects of Maxwell stress and hyperelasticity. The Maxwell stress $p$ on the DE membrane is given by~\eref{eqn:DEAstrain}~\cite{Pelrine_1998_DEA}:
\begin{equation}
    \label{eqn:DEAstrain}
    p = {e_0e_r}\Big(\frac{V}{z}\Big)^2
\end{equation}

where $V$ is the applied voltage across thickness $z$ of the DE membrane. The relative permittivity is $e_r$, and the permittivity of free space is $e_0$. To model the non-linear elastic behaviour, recent works utilize hyperelastic material models, such as the Gent and the Neo-Hookean models~\cite{Zhang_2019_DEAnonlinear}. However, this hyperelastic  behaviour reduces to linearly elasticity for small strains ($\leq10\%$), which is the case for thin membranes.

%%%%%%%%%%%%%%%%%%%%%%%%%%%%%%%%%%%%%%%%%%%%%%%%%%%%%%%%%%%%%%%%%%%%%%%%%%%%%%%%
\paragraph{Finite Element Methods (FEM)}
\label{sec:DEMaterialFEM}
%%%%%%%%%%%%%%%%%%%%%%%%%%%%%%%%%%%%%%%%%%%%%%%%%%%%%%%%%%%%%%%%%%%%%%%%%%%%%%%%
FEM is a numerical method for solving differential equations and mathematical modeling of a physical system. To model DE material in FEM, we approximate their behaviour using piezoelectric materials elements~\cite{Piefort_2000_FEMPeiso}, as there are no commercial FEM packages that provide DE elements as standard. We modify the piezoelectric finite elements material properties to model the Maxwell stress effect observed in dielectric materials. These elements assume linear elasticity, which is not a limiting factor as we can assume such behaviour for our case of thin DE membranes~\cite{Araromi_2012_FEMDEA}. Similar to DE, piezoelectric materials exhibit strain when in the presence of electric fields. The piezoelectric stress is given by~\eref{eqn:peizoelectricstress}.
\begin{equation}
\label{eqn:peizoelectricstress}
\sigma_{ij} = D^E_{ijkl}\epsilon_{kl} - e_{mij}E_m
\end{equation}

where elastic stiffness matrix is $D^E_{ijkl}$, the strain tensor is $\epsilon_{kl}$, the piezoelectric stress coefficient is $e_{mij}$ and the electric potential gradient is $E_m$. As detailed in~\cite{Araromi_2012_FEMDEA} the piezoelectric stress becomes approximately equal to the Maxwell stress for a thin membrane, such that the strain $e_{zz}$ in the direction of thickness ($z$-axis) in the DE membrane is given by (subscript z - $z$-axis, for details see~\cite{Araromi_2012_FEMDEA}):
\begin{equation}
\label{eqn:peizoelectricstrain}
e_{zz} = e_re_0E_z
\end{equation}
